# Supplementary material for: Towards Multi-Agent Reinforcement Learning using Quantum Boltzmann Machines
Source: arXiv:2109.10900 source file (2021-11-22)
Supplement: Supplementary file 1 [file appendix.tex]

\newpage
\appendix
\section{Appendix}\label{appendix}

\subsection{Parameters Used}
All parameters stayed the same throughout the whole evaluation.

\begin{table}[!hb]
  \centering
  \label{parameters}
  \begin{tabular}{c|c|l}
    \toprule
    Parameter&Description&Value\\
    \midrule
    nb\_steps & Step boundary per episode& 2000\\
    nb\_episodes & Number of episodes per run& 500\\
    nb\_runs\_per\_env& Number of runs per experiment & 10\\
    lr & Learning rate weight updates & 0.005\\
    discount_factor & Discount of future rewards & 0.8\\
    epsilon\_min & Minimum exploration rate & 0.1\\
    epsilon\_decay & Exploration decay per training step & 0.0008\\
    mini\_batch\_size & Mini batch size & 8\\
    warm\_up & Steps before first weight update & 250 \\
    target\_update & Update period of target network & 250 \\
    memory\_size & Size of ERB & 20000\\
    replica\_count & Number of QBM replicas & 1\\
    average\_size & Number of configurations per replica & 10\\
    num\_sweeps & Number of steps & 1000\\
    \bottomrule
\end{tabular}\\\\
\caption{Parameter setting for the reinforcement learning loop, ERB and QBM agent.}
\end{table}
\newpage
\subsection{Q-RL Pseudo-Code}\label{pseudo}
\begin{algorithm}[H]
\SetAlgoLined
\SetKwInOut{Input}{Input}
 \For{$episode$ $e \leftarrow 0$ \textbf{to} $E$}{
 \For{\textit{time step} $t \leftarrow 0$ \textbf{to} $T$}{
 Sample actions $a^{i}_{t}$ from policies $\pi^{i}$ for each agent $i$ in state $s_{t}$\;
  \For{each agent i}{
    Get observations $s^{i}_{t+1}$ and rewards $r^{i}_{t}$ by applying $a^{i}$\;
 Store $e^{i}_{t} \leftarrow \langle s^{i}_{t}, a^{i}_{t}, r^{i}_{t}, s^{i}_{t+1} \rangle$ for $E^{i}$ for each agent $i$\;
  Update weights to refine $\pi^{i}$ on the basis of $E^{i}$ for each agent $i$\;}
   Set $s_{t} \leftarrow s_{t+1}$
 }}
 \SetKwProg{Procedure}{Procedure}{}{}
 \Procedure{Weight Update}{
  \For{batch $i$ in mini-batch}{
    Calculate $-F(s^{i}_{t}, a^{i}_{t})$ with policy network\;
    Calculate $max(-F(s^{i}_{t+1}, a))$ with target network\;
    Set $Q(s^{i}_{t}, a^{i}_{t}) \leftarrow -F(s^{i}_{t}, a^{i}_{t})$\;
    Set $Q(s^{i}_{t+1}, a) \leftarrow max(-F(s^{i}_{t+1}, a))$\;
    Update policy network based on $Q(s^{i}_{t}, a^{i}_{t})$ and $Q(s^{i}_{t+1}, a)$\;
    \If{time step (mod update-period) = 0}{
    Set target network $\leftarrow$ policy network\;}}
 }
 
 \caption[Pseudo-Code for Q-RL]{Pseudo-Code for Q-RL}
 \label{new_code}
\end{algorithm}
